# Supplementary material for: Catastrophic-risk-aware reinforcement learning with extreme-value-theory-based policy gradients
Source: arXiv:2406.15612 source file (2024-06-28)
Supplement: Supplementary file 1 [file Online_appendix.tex]

\centerline{\Large \textbf{Online Appendix (not part of the paper)}}

\section{BLABLA}
